# Supplementary material for: Differentiable Ranks and Sorting using Optimal Transport
Source: arXiv:1905.11885 source file (2019-11-02)
Supplement: Supplementary file 1 [file appendix.tex]

\newpage
\section{Appendix}

Jacobian of $J_{\bx}\opScdf{\ba,\bx}{\bb,\by}$ as $\ell\rightarrow \infty$.

We write everything as a function of $\bx$. We write $K(\bx)=e^{-c(x_i,y_j)/\varepsilon}$.

Upon termination of Sinkhorn iterations one has
$$u(\bx) \circ K v(\bx) = \ba, \quad u v(\bx) \circ K^T u(\bx) = \bb.$$
We simplify this expression by writing 
$$ w(x)\eqdef \begin{bmatrix}u(\bx)\\v(\bx)\end{bmatrix},
\;
\bc\eqdef \begin{bmatrix}\ba\\ \bb\end{bmatrix},\quad \Lambda(\bx)\eqdef 
\begin{bmatrix} 
\mathbf{0}_{n\times n} & K(\bx)\\ K(\bx)^T & \mathbf{0}_{m\times m}
\end{bmatrix}, $$

Writing
$$f(\bx,\bz)=\bz\circ \Lambda(\bx) \bz - \bc,$$ one has upon convergence that,  $f(\bx,w(\bx))=0$. The implicit function theorem states in that case that

$$J_{\bx} w(\bx) = - \left[J_{\bz} f(\bx,\omega(\bx))\right]^{-1} J_{\bx}f(\bx,\omega(\bx))\in\mathbb{R}^{(n+m)\times n}$$

To compute the action of the first operator, one can use simple differential calculus to get that the application of the first Jacobian to an infinitesimally small vector $\bh$ is equal to:

$$\left(J_{\bz} f(\bx,\bz) \right) \bh = f(\bx,\bz+\bh)-f(\bx,\bz)= \bh\circ\Lambda(\bx)\bz + \bz\circ \Lambda(\bx)\bh$$

Therefore if one is interested in applying the inverse of that operator, one has that if $J_{\bz} [f(\bx,\bz)] \bh = \bg$, then 
$$\bg = \bh\circ\Lambda(\bx)\bz + \bz\circ \Lambda(\bx)\bh$$
which yields
$$\frac{\bg}{\bz}= \bh\circ\frac{\Lambda(\bx)\bz}{\bz} + \Lambda(\bx)\bh$$
and therefore
$$\frac{\bg}{\bz} = \left(\diag\left(\frac{\Lambda(\bx)\bz}{\bz}\right) + \Lambda(\bx)\right)\bh$$ yielding
$$\left(J_{\bz} [f(\bx,\bz)]\right)^{-1}= \left(\diag\left(\frac{\Lambda(\bx)\bz}{\bz}\right) + \Lambda(\bx)\right)^{-1}\diag(\bz^{-1}),$$
which, reverting to our notations, can be seen as

$$\left(\begin{bmatrix}\diag\left(\frac{K(\bx) v(\bx)}{u(\bx)}\right)&K(\bx)\\K^T(\bx)& \diag\left(\frac{K^T(\bx) u(\bx)}{v(\bx)}\right)\end{bmatrix}\right)^{-1}\diag\left(\begin{bmatrix}u(\bx)^{-1}\\v(\bx)^{-1}\end{bmatrix}\right) = 
\left(\begin{bmatrix}\diag\left(K(\bx) v(\bx)\right)&\diag(u(\bx))K(\bx)\\\diag(v(\bx))K^T(\bx)& \diag\left(K^T(\bx) u(\bx)\right)\end{bmatrix}\right)^{-1}
$$

On the other hand, 
$J_{\bx}f(\bx,\omega(\bx))=\begin{bmatrix}\diag(u(\bx))\circ \Delta v(\bx)\\\diag(v(\bx))\Delta^T \diag(u(\bx))\end{bmatrix}\in\mathbb{R}^{(n+m)\times n}$

where $\Delta=\left[-\frac{c'_x(x_i,y_j)}{\varepsilon}e^{-\frac{c(x_i,y_j)}{\varepsilon}}\right].$

Hence, we obtain that 

$$J_{\bx} w(\bx) = - \left[J_{\bz} f(\bx,\omega(\bx))\right]^{-1} J_{\bx}f(\bx,\omega(\bx))\in\mathbb{R}^{(n+m)\times n}$$
